# Supplementary material for: Magnetic ground states of honeycomb lattice Wigner crystals
Source: arXiv:2206.10024 source file (2022-06-20)
Supplement: Supplementary file 1 [file Supplemental_paper.pdf]

**SUPPLEMENTARY INFORMATION** for

# Magnetic ground states of honeycomb lattice Wigner crystals

by N. Kaushal, N. M. Durán , A. H. MacDonald, and E. Dagotto

## I. MAGNETIC STATES IN THE WEAK AND INTERMEDIATE $U_0/t$ REGION

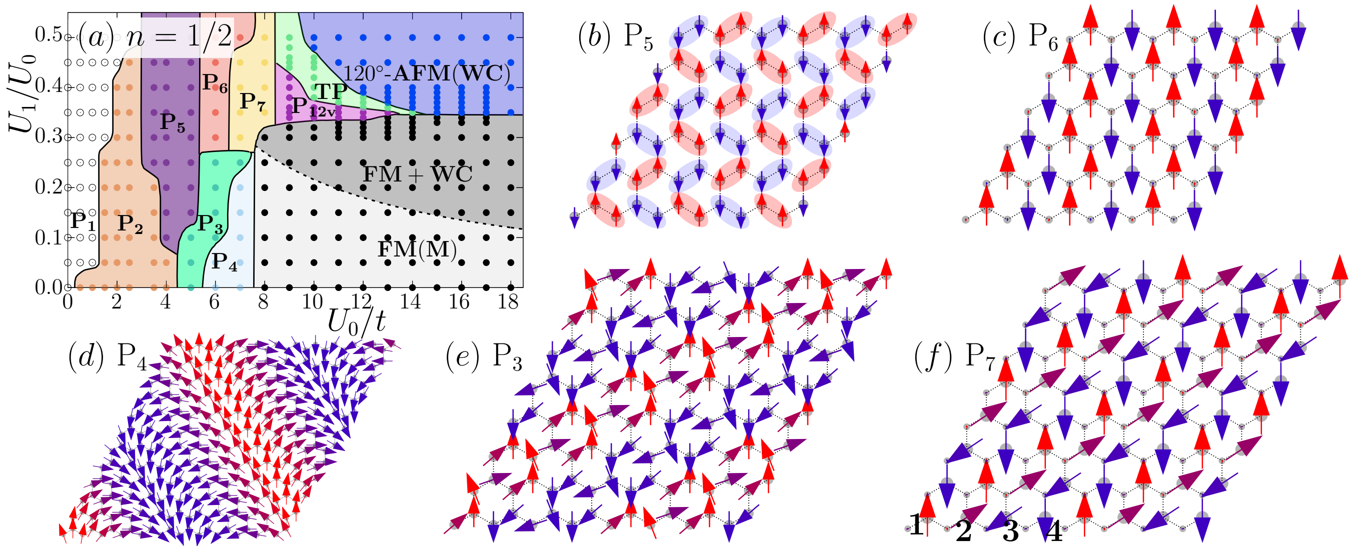


FIG. 1: In panel (a), the $U_1/U_0$ vs $U_0/t$ phase diagram is shown, fixing $d = 10a_m$. Panels (b,c,d,e,f) show representative states for the phases $P_5, P_6, P_4, P_3$, and $P_7$, respectively

.

$n = 1/2$ **results:** In this subsection we will discuss the states we found for filling $n = 1/2$ in the weak and intermediate $U_0/t$ region, which were not discussed in the main text. We show the phase diagram in Fig.1(a), including the $U_0 < 10t$ region. Phase $P_1$ is the trivial paramagnetic metal which is stable only in the weak $U_0$ region, we noticed its stability increases on increasing $U_1/U_0$ probably due to renormalization of bands.

At fixed $U_1/U_0 = 0$, first we found the $P_2$ phase which is a homogenous ferromagnetic phase with a very weak net magnetization of $\approx 0.08$ (i.e. "partially" ferromagnetic). This state can be attributed to the Stoner magnetism. Increasing $U_0/t$ further, we found unexpected phases, such as $P_3$ and $P_4$. Phase $P_3$, see Fig. 1(e), is an AFM bistriped state where one stripe is made up of chains of hexagons displaying bented ferromagnetism, while the other stripe has exactly the opposite spins with respect to the first stripe. Phase $P_4$ is a planar spiral phase, shown in Fig.1(d), which is present in the vicinity of the fully polarised large-$U_0$ FM metallic state. This planar spiral phase was also found in Hartree-Fock calculations of the triangular lattice [1].

Near the $U_0 \approx 4.0t$ region, we noticed, on increasing $U_1/U_0$, the system transits to an AFM phase with 2-site dimers, shown in Fig.1(b) (named $P_5$). The $P_5$ phase is also present as a ground state of the double-exchange models on a honeycomb lattice [2] as a "trade-off" between AFM and FM states, which is consistent with our findings as well because this state is "sandwiched" between Stoner FM state and the large $U_0$ AFM states. We noticed for the large values of $U_1/U_0$, for any $U_0 \gtrsim 6$, the Wigner crystallization into an the emergent triangular lattice is favored for robust values of $U_1/U_0$. Near $U_0 \approx 6t$, for $U_1/U_0 \gtrsim 0.3$ we found the triangular Wigner Crystal phase with zig-zag AFM ordering shown in Fig. 1(c), named $P_6$ . This Zig-Zag AFM ordering in triangular lattice has already been reported as the stable state in the intermediate onsite $U_0/t$ region in the mean-field calculations on half-filled triangular lattices [3]. We also observed a novel 4-sublattice *non-collinear* AFM state, named $P_7$, see Fig. 1(f)) where the spins "1" and "4" as well as the spins "2" and "3" are antiparallel, but the spins "1" and "2", as well as "3" and "4", are at nearly 60°. We noticed the angle between "1(3)" and "2(4)" reduces from 60° to 0° as $U_1/U_0$ increases and eventually phase $P_7$ smoothly transists into the zigzag $P_6$ state. The rest of the large-$U_0/t$ states have been already discussed in the main text. Those states are the ones primarily relevant for the Moiré materials.

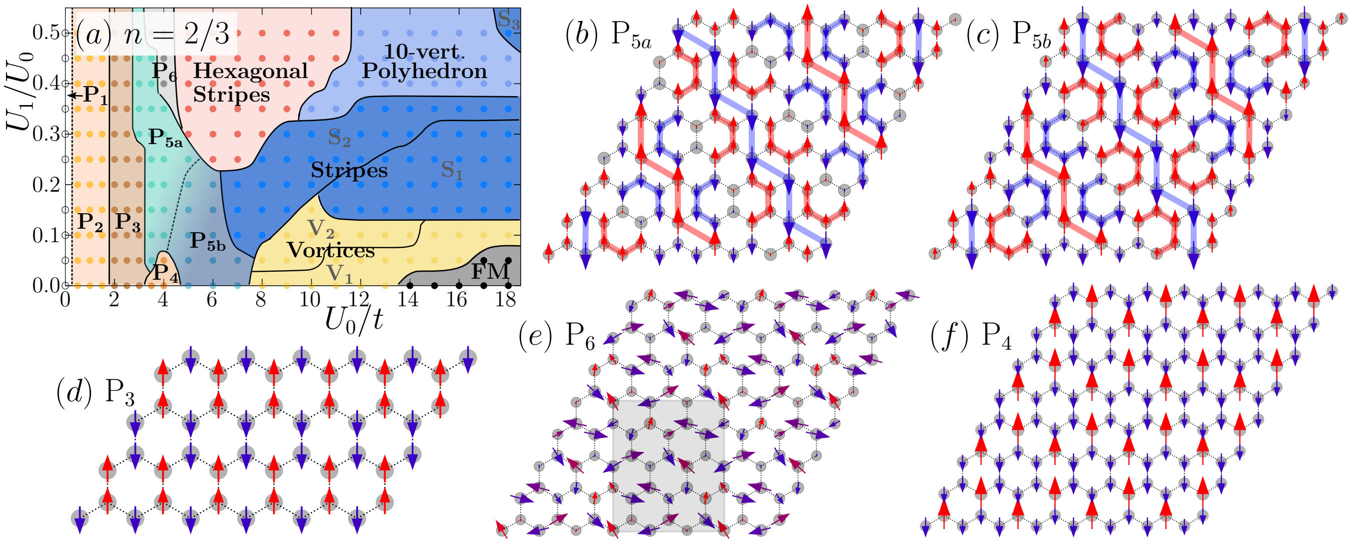


FIG. 2: In panel (a), the $U_1/U_0$ vs $U_0/t$ phase diagram is shown, fixing $d = 10a_m$. Panels (b,c,d,e,f) show representative states for the phases $P_{5a}, P_{5b}, P_3, P_6$, and $P_4$, respectively

$n = 2/3$ **results:** Figures 2(b-f) show the representative states of the phases present in the weak and intermediate $U_0/t$ strength region at $n = 2/3$, with the complete phase diagram shown in Fig. 2(a). The $P_1$ region is a canonical paramagnetic metal present in a narrow region around $U_0/t = 0$. We noticed a feeble ferromagnetic phase that develops rapidly as $U_0$ is increased from zero, with small net magnetization $|m| \approx 0.026$. On further increasing $U_0/t$, AFM states start appearing, similar as in the $n = 1/2$ case. Phase $P_3$ has 2-site FM stripes aligned opposite to each other, as shown in Fig. 2(d). Near the line $U_1/U_0 = 0$, we found a small region of phase $P_4$ having a honeycomb lattice of $\uparrow$ spins with lattice spacing $2a_m$ and $\downarrow$ spins embedded inside the hexagons of the $\uparrow$ spins, see Fig. 2(f). In the $U_0/t \in [4, 8]$ region, we found the $P_{5a(b)}$ phases which are smoothlty connected to each other. A representative state of the $P_{5a}$ phase is shown in Fig. 2(b) having zig-zag FM chains of $\uparrow$ and $\downarrow$ spins separated by 4-site arcs and two sites with nearly 0 local moment. Increasing $U_0/t$ leads to the development of the moment on the sites initially having nearly 0 moment, state that we call phase $P_{5b}$ (see Fig. 2(c)).

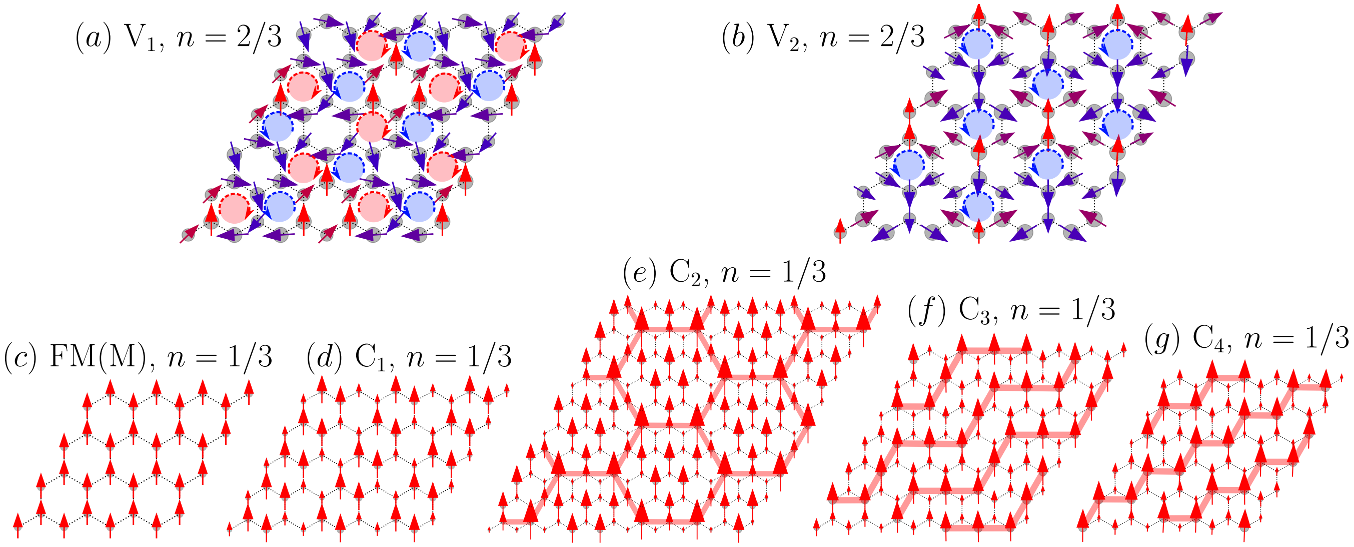


FIG. 3: States for Vortices phases for the filling $n = 2/3$ are shown in panels (a,b). Panel (c) show the FM+Metal state, and panels (d-g) show the FM+CDW states present in the $n = 1/3$ phase diagram

On further increasing $U_0/t$, phase $P_{5b}$ transists into the phase $S_2$ (shown already in the main text) as Wigner crystallization sets in as dominant tendency. Figure 2(e) shows a representative state for phase $P_6$, present near

$U_0/t \approx 4.0$ and large $U_1/U_0$ but capturing only a small portion of the phase diagram. The magnetic unit cell is shown via the grey colored box, inside which the spins are pointing in multiple directions. As discussed in the main paper, we also found Vortices phases named $V_1$ and $V_2$ here. In these phases the electronic spins either orient clockwise or anti-clockwise making the 6-site hexagon vortices. In the $V_1$ phase we found staggered ordering of this vortices, see Fig. 3(a), and whereas the $V_2$ phase has homogenous vorticity (see Fig. 3(b)).

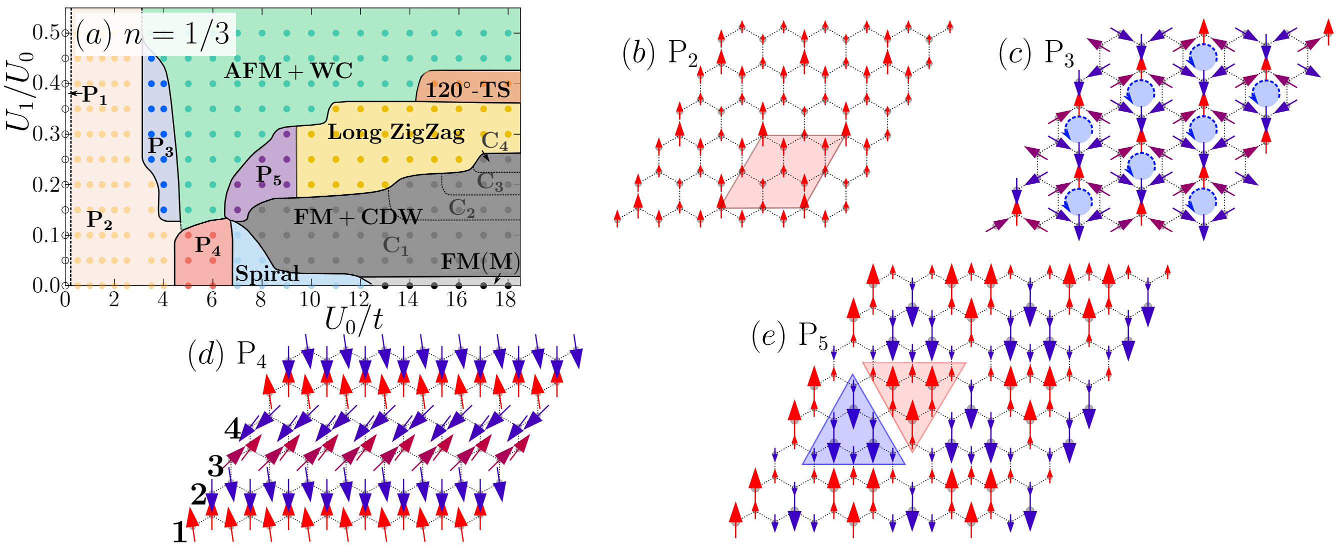


FIG. 4: In panel (a), the $U_1/U_0$ vs $U_0/t$ phase diagram is shown, fixing $d = 10a_m$. Panels (b,c,d,e) show representative states for the phases $P_2, P_3, P_4$, and $P_5$, respectively

$n = 1/3$ **results:** The results at $n = 1/3$ are shown in Fig. 4, with the phase diagram shown in Fig. 4(a). Phases $P_1$ and $P_2$ are the trivial paramagnetic metal and the weak FM phase, respectively. Interestingly we noticed that the $P_2$ phase also has tendencies towards a weak charge density wave with a new unit cell having lattice vectors $2\mathbf{a_1}$ and $2\mathbf{a_2}$, see Fig. 4(b) for an illustration. In the small $U_1/U_0$ region, for instance $U_1/U_0 = 0$ as special case, and for $U_0/t \in [5, 12]$ *non-collinear* states were found, namely the $P_4$ and Spiral states. The $P_4$ phase has 4 distinct FM zig-zag stripes with small benting (see Fig. 4(d)), where the stripes "1" and "2", as well as "3" and "4" are aligned opposite to each other, while stripes "2(1)" and "3(4)" are at nearly 60° with respect to each other. The planar spiral phase is similar to phase $P_4$ of $n = 1/2$ (shown in Fig. 1(d)). Near $U_0/t = 4$, at the intermediate $U_1/U_0$ region, we found a phase with 6-sublattice state where the electronic spins makes vortex structure on hexagons, named $P_3$, shown in Fig. 3(c). We also noticed an exotic phase with FM triangular clusters of both $\uparrow$ and $\downarrow$ spins, named $P_5$, shown in Fig. 3(e).

Finally, we also show the representative states for the FM region present in the large $U_0/t$ region, see Fig. 3(c-g). We found 4 type of charge density waves in FM region (at finite value of $U_1/U_0$), named $C_1$, $C_2$, $C_3$, and $C_4$, in the order of increasing $U_1/U_0$. We noticed that these CDW's are weak, specially for the low values of $U_1/U_0$, so in the Fig. 3(d-g) the red arrows and grey circles are proportional to $|\langle \mathbf{S}_i \rangle|^2$ and $\langle n_i \rangle^2$, respectively (instead of $|\langle \mathbf{S}_i \rangle|$ and $\langle n_i \rangle$ as in rest of the paper), for the clear visibility of the CDW patterns. The $C_1$ phase has 2-site thick FM stripes, see Fig. 3(d), and it appears first as soon as $U_1/U_0$ becomes non-zero. This phase covers the majority of the FM region. Further increasing $U_1/U_0$ we found a honeycomb FM+CDW phase ($C_2$), see Fig. 3(e), with a lattice spacing of $2a_m$, and later we observed the $C_3$ 3-sites and $C_4$ 2-sites zigzag FM stripes shown in Figs. 3(f) and (g), respectively.

## II. CHIRALITY OF NON-COPLANAR STATES AT $n = 1/2$

In Figure 5, the chirality $\chi_{ijk} = \mathbf{S}_i \cdot (\mathbf{S}_j \times \mathbf{S}_k)$ for the Trigonal Prism (TP) and 12-vertices polyhedron ($P_{12v}$) states is shown, where the $i, j, k$ are the sites on the triangular lattice Wigner crystal. As discussed in the main text, we found that the net chirality $\chi = \sum_{\triangle} \chi_{ijk}$ (sum over all triangular plaquettes) of both of the TP and $P_{12v}$ states is zero. Moreover, the state TP has stripe order in the chirality (see Fig. 5(a)) while the state $P_{12v}$ also has stripes of positive and negative $\chi_{ijk}$ but made up of hexagons (see Fig. 4(5)), again canceling out each other.

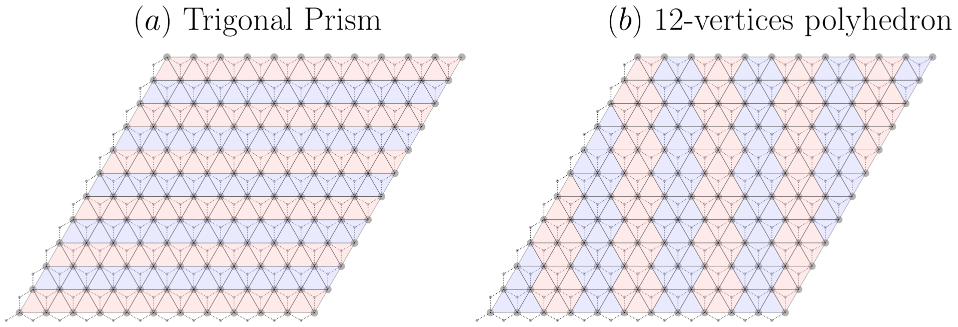


FIG. 5: The chirality for all triangular plaquettes in the triangular lattice Wigner crystal is shown for the *non-coplanar* Trigonal Prism and 12-vertices polyhedron states in panel (a) and (b), respectively. The blue and red color implies $\chi_{ijk} > 0$ and $\chi_{ijk} < 0$, respectively.

## III. DENSITY OF STATES FOR $n = 2/3$ IN LOW $U_1/U_0$ REGION

As mentioned in the main paper, we used the single particle density of states ($\rho(\omega)$) to attain the metal-insulator transition line shown in the large $U_0$ phase diagrams (Fig.4(a,b) in the main-paper) of $n = 2/3$. Here, we will discuss the $\rho(\omega)$ for few points from $n = 2/3, d = 10a_m$ phase diagram, particularly for the low $U_1/U_0$ values fixing the system size to $48 \times 48$. We used the self-consistently converged solution of $12 \times 12$ system to calculate the $\rho(\omega)$ for the $48 \times 48$ system, to overcome the finite-size effects in density of states. In Fig. 6(a), we show the $\rho(\omega)$ for $U_1/U_0 = 0.05$, 0.1, and 0.15 values (fixing $U_0 = 12t$). It is evident that for $U_1/U_0 = 0.05$ and $U_0 = 12t$, there is '$V$'-shaped gap at chemical potential ($\mu$), making the system metallic, whereas for $U_1/U_0 = 0.05$ and 0.1 we found a robust '$U$'-shaped gap suggesting an insulating state. We also show $\rho(\omega)$ for the same $U_1/U_0$ points, but fixing $U_0 = 30t$, see Fig.6(b). For the $U_1/U_0 = 0.05$ and $U_0 = 30t$, we notice only a small suppresion in the density of states at chemical potential making it a metallic state, whereas a clear gap for $U_1/U_0 = 0.05$ and 0.1 values. We performed similar analysis for all the points in the phase diagram in the region of $U_0 >= 10t$ and $U_1/U_0 <= 0.2$, to achieve the metal-insulator transition line shown in the main paper.

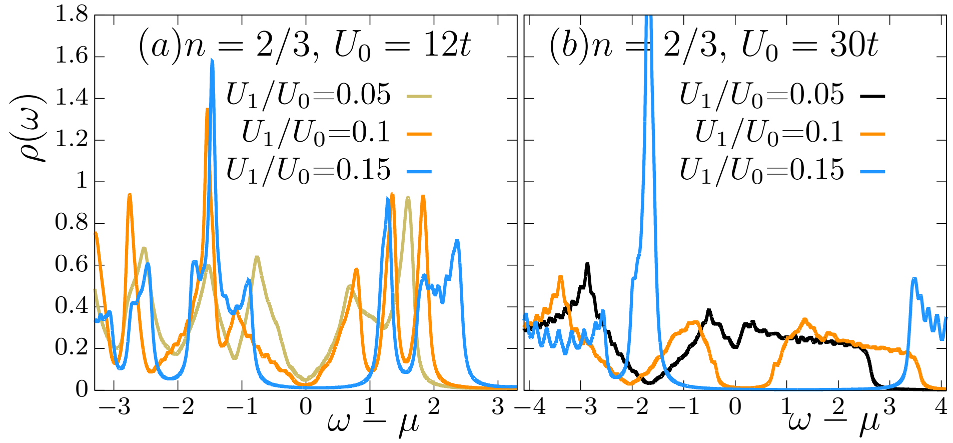


FIG. 6: Panels (a) and (b) show the single particle density of states $\rho(\omega)$ for filling $n = 2/3$, for $U_1/U_0 = 0.05$, 0.1, and 0.15, at fixed $U_0 = 12t$ and $U_0 = 30t$, respectively.

## IV. MAGNETIZATION EVOLUTION FOR $n = 1/3$ AND $n = 2/3$ WIGNER CRYSTALS

In this section we discuss the magnetization $|m|$ evolution with the external magnetic field ($h/t$) for the $n = 1/3$ and $n = 2/3$ Wigner crystal states, fixing $d = 10a_m$. In Fig. 7(a), we show results for $n = 2/3$ in the large $U_1/U_0$ region, particularly $\{U_1/U_0, U_0/t\} = \{0.4, 12\}$ and $\{0.45, 12\}$ as representative points of 10-vertices polyhedron phase

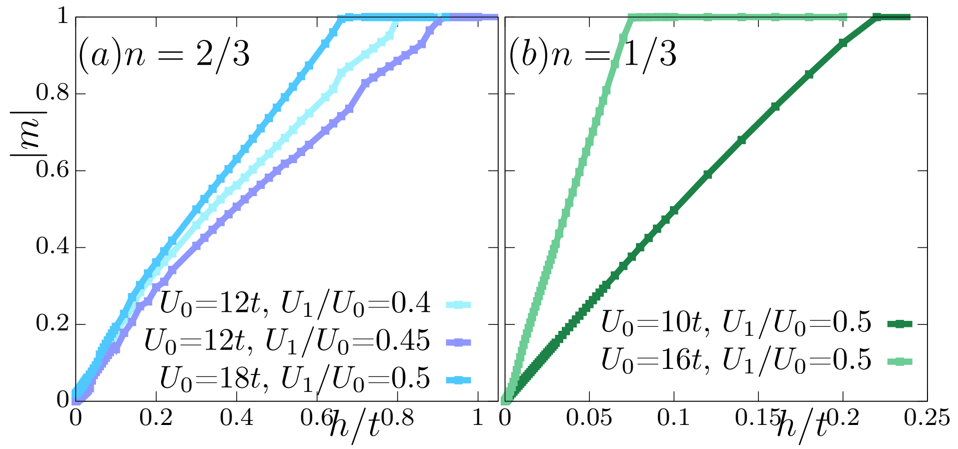


FIG. 7: The magnetization $|m|$ vs magnetic field $h/t$ curves are shown for the Wigner states for fillings $n = 2/3$ and $n = 1/3$ in panels (a) and (b), respectively.

and $U_1/U_0 = 0.5$, $U_0 = 18t$ as a representative point of $S_3$ phase. We also show the $|m|$ vs $h/t$ curves for $n = 1/3$ in Fig. 7(b) for the points $\{U_1/U_0, U_0/t\} = \{0.5, 10\}$ and $\{0.5, 16\}$ belonging to AFM+WC phase (see $n = 1/3$ Phase diagram). We noticed that for all above states, magnetization increases continuously by canting the $h = 0$ state and without occurrence of any fractional magnetization platues unlike to $n = 1/2$ case (shown in the main paper).

Interestingly the saturation magnetic field for $n = 2/3$ is much larger than $n = 1/2$ and $n = 1/3$ states because in the $n = 2/3$ Wigner crystal the nearest neighbour superexchange is present whereas for $n = 1/2$ and $1/3$ the much weaker next-nearest neighbour exchange is the dominant energy scale.

## V. HOPPING PARAMETERS ESTIMATES FOR THE TIGHT BINDING MODEL

We calculated the hopping parameters for tight-binding model, using the top-most band i.e. closest to the chemical potential, from the band-structure calculated by the continuum model (see Fig. 1 of the main paper). In Fig. 8, we show the nearest-neighbour $t_1$ and the next-nearest neighbour $t_2$ hopping parameter values for twisted $MoSe_2$ homobilayer. We found that $t_1/t_2 < 0$ for any value of the twist angle ($\theta$) and the bandwidth increases by increasing the ($\theta$) (both $|t_1|$ and $|t_2|$ increases). We noticed that $|t_1/t_2| \in \{800, 10\}$ for $\theta \in \{1.0°, 3.0°\}$; because of relatively negligible values of $t_2$, specially for small twist angles, we ignored the next-nearest neighbour hoppings in our calculations.

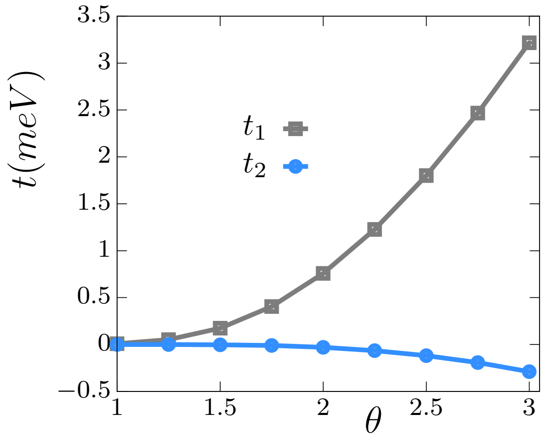


FIG. 8: The nearest neighbour $t_1$ and the next-nearest neighbour $t_2$ hopping parameters on honeycomb Moiré lattice are shown for twisted $MoSe_2$ homobilayer, for various values of twist angles ($\theta$).

[1] K. Pasrija and S. Kumar, Phys. Rev. B **93**, 195110 (2016).
[2] J. W. F. Venderbos, M. Daghofer, J. van den Brink, and S. Kumar, Phys. Rev. Lett. **107**, 076405 (2011).
[3] L.-F. Lin, N. Kaushal, C. Şen, A. D. Christianson, A. Moreo, and E. Dagotto, Phys. Rev. B **103**, 184414.
